# Supplementary material for: MIMO for MATLAB: A Toolbox for Simulating MIMO Communication Systems
Source: arXiv:2111.05273 source file (2021-11-09)
Supplement: Supplementary file 1 [file sec-appendix.tex]

\appendices

\section{Example: A Four-Device Interference Network}

\subsection{Description}
In this example, we demonstrate \mfm's ability to handle interference when two links attempt to coexist using the same radio resources.
Consider the network shown in \figref{fig:example-01}, where four fully-digital transceivers are present.
Tx-1 transmits to Rx-1, and Tx-2 transmits to Rx-2.
Tx-1 and Rx-1 are separated by $100$ meters.
Tx-2 and Rx-2 are also separated by $100$ meters.
The two pairs are separated by $100$ meters between them in the $x$ direction as shown, introducing inter-user interference.

All devices operate using the same radio resources, leading to interference from Tx-1 onto Rx-2 and from Tx-2 onto Rx-1.
All devices operate using $0$ dBm of transmit power over a symbol bandwidth of $50$ MHz at $5$ GHz. 
The noise power at each receiver is $-174$ dBm/Hz.
Transmitters use $4$ antennas and receivers are equipped with $8$ antennas. 
Suppose $4$ streams are being multiplexed by each device.
Let all channels be Rayleigh-faded and the path loss follow free-space path loss with an exponent of $2$.

\begin{figure}[t]
	\centering
	\includegraphics[width=\linewidth,height=0.4\textheight,keepaspectratio]{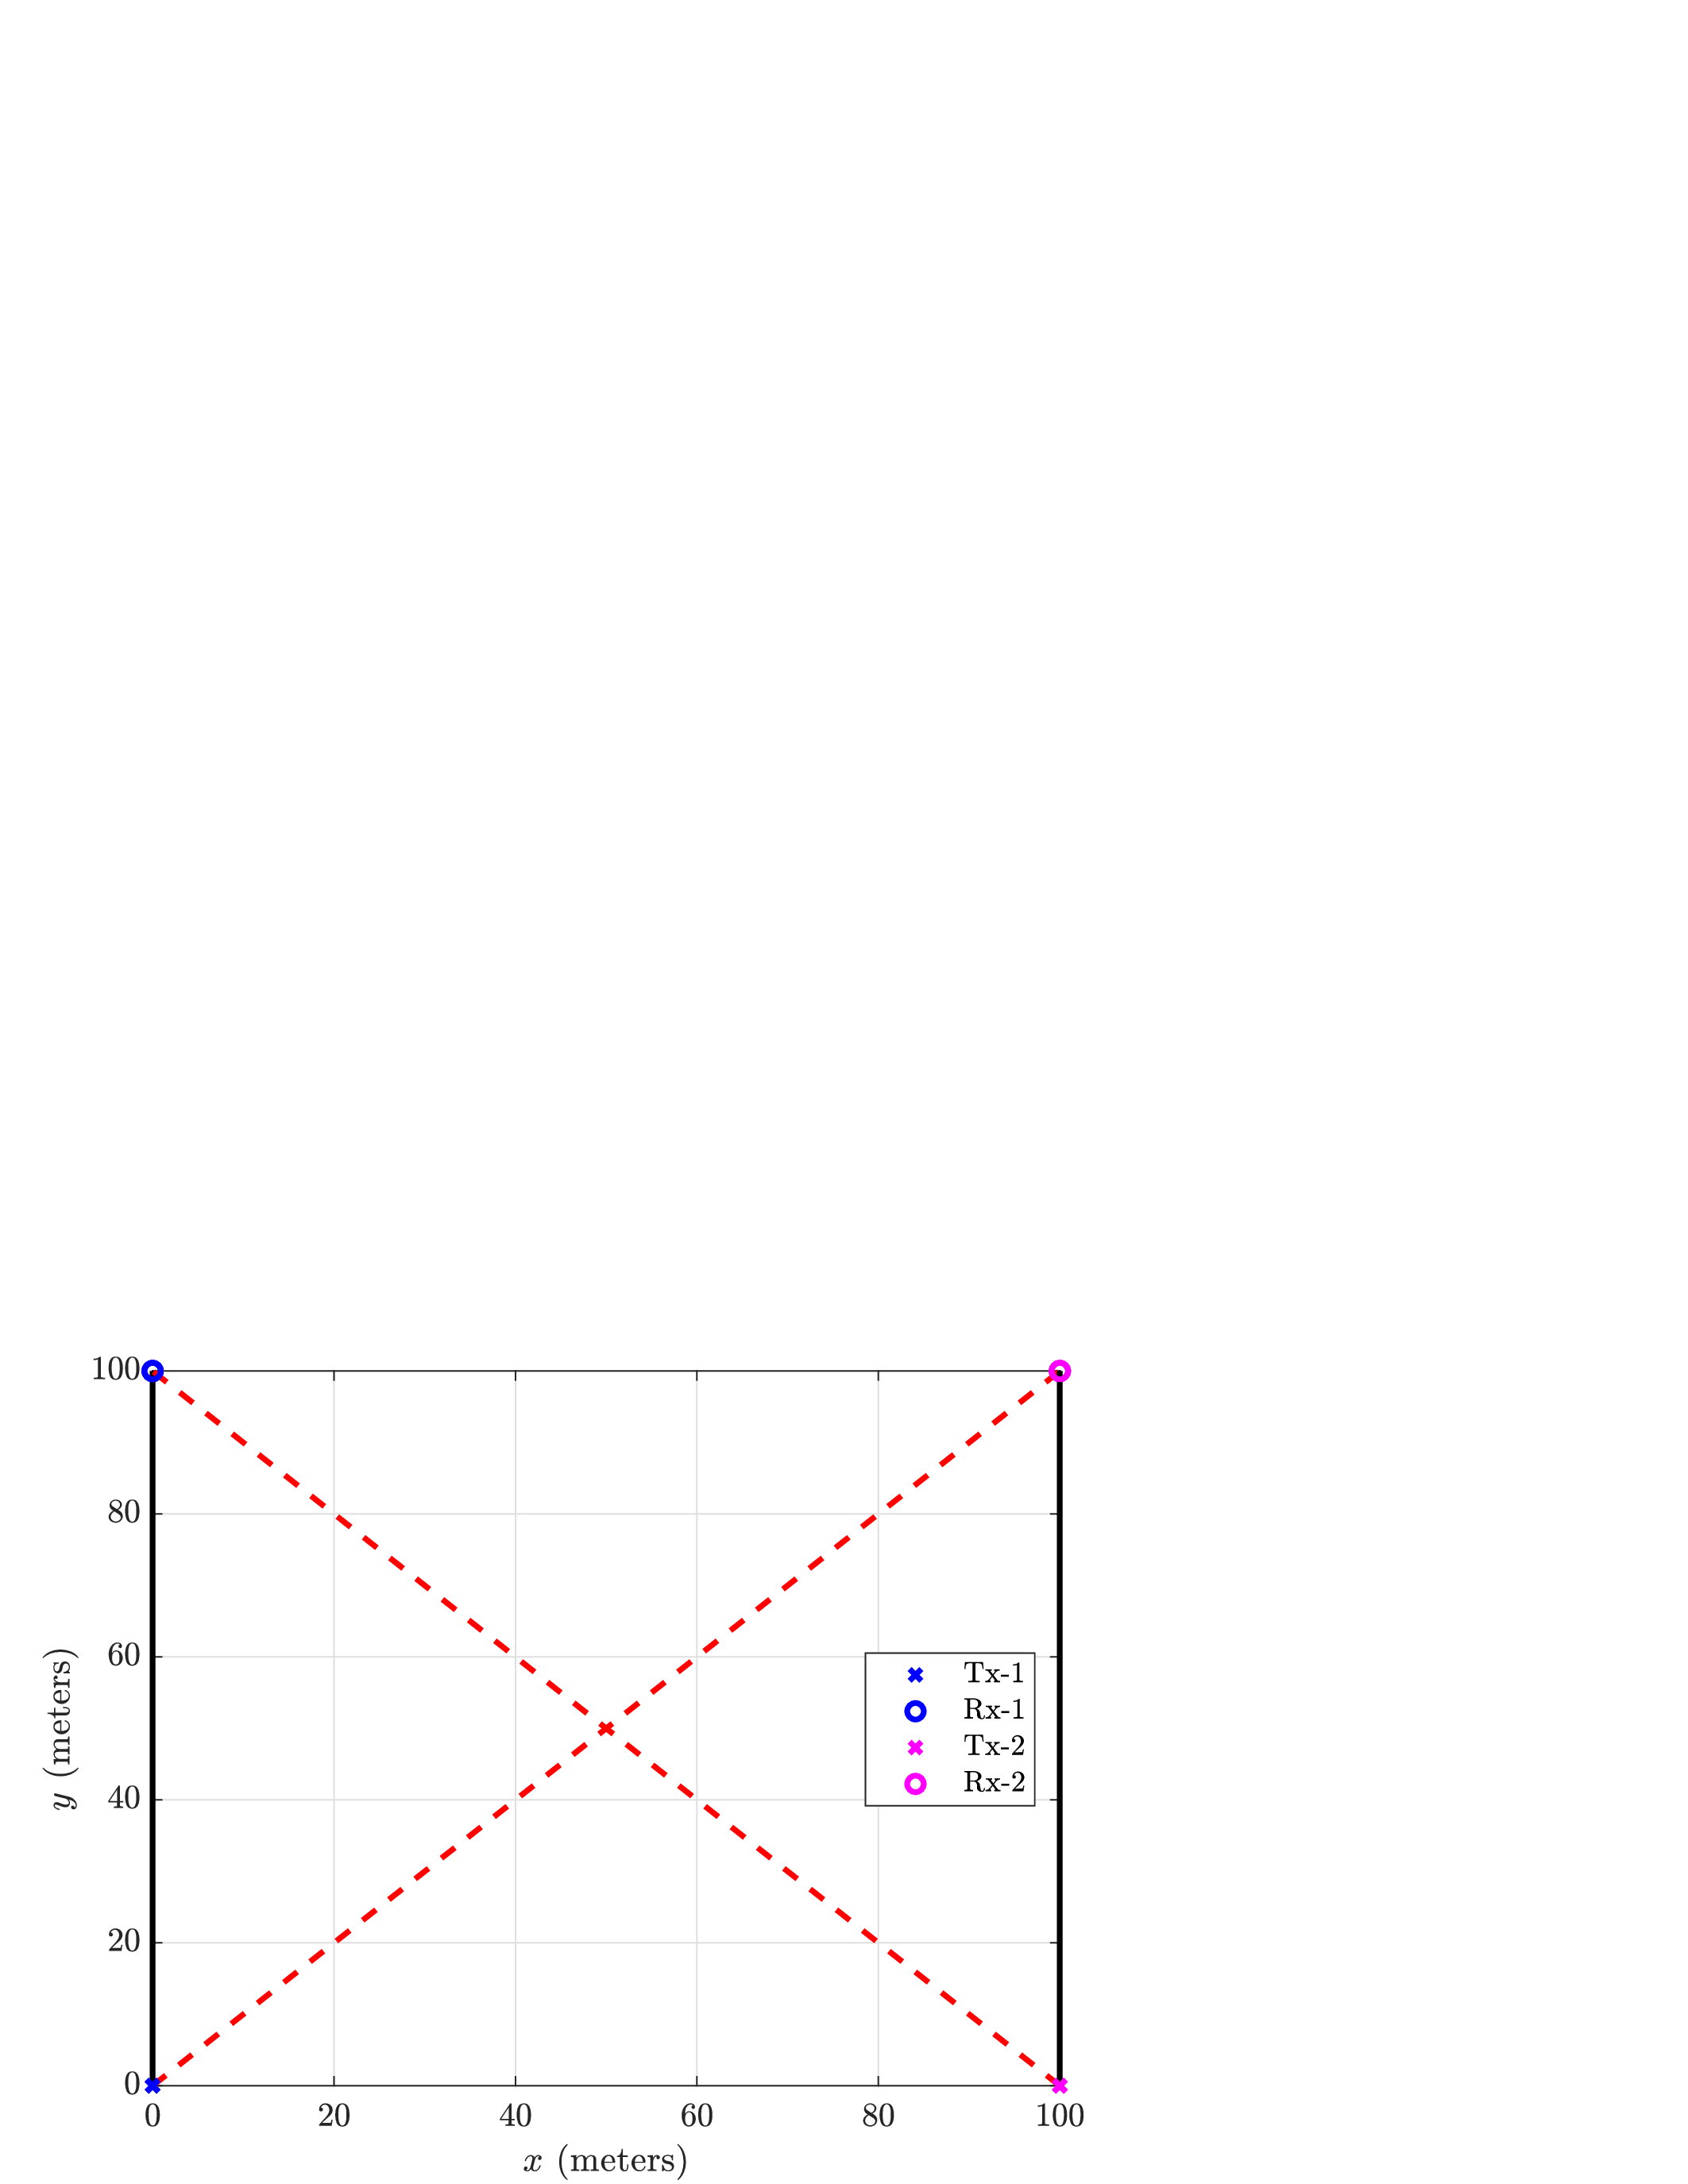}
	\caption{The network of four devices simulated used in example 1.}
	\label{fig:example-01}
\end{figure}

\subsection{MFM Implementation}

\begin{verbatim}
clc; clearvars; close all; rng(99);

% System variables.
symbol_bandwidth_Hz = 50e6;
carrier_frequency_Hz = 5e9;
propagation_velocity_meters_per_sec = 3e8;
noise_power_per_Hz_dBm_Hz = -174;
num_streams = 4;
transmit_power_dBm = 0;
Nt = 4;
Nr = 8;

% Create some template transmit and receive arrays to use.
array_transmit_object = array.create(Nt);
array_receive_object = array.create(Nr);

% Create and setup a template device.
device_object = device.create('transceiver','digital');
device_object.set_arrays(array_transmit_object,array_receive_object);

% Channel object.
channel_object = channel.create('Rayleigh');

% Path loss object.
path_loss_object = path_loss.create('free-space');
path_loss_object.set_path_loss_exponent(2);

% Create our device instances.
dev_1 = copy_object(device_object);
dev_1.set_name('Tx-1');
dev_1.set_coordinate([0,0,0]);
dev_1.set_marker('bx');

dev_2 = copy_object(device_object);
dev_2.set_name('Rx-1');
dev_2.set_coordinate([0,100,0]);
dev_2.set_marker('bo');

dev_3 = copy_object(device_object);
dev_3.set_name('Tx-2');
dev_3.set_coordinate([100,0,0]);
dev_3.set_marker('mx');

dev_4 = copy_object(device_object);
dev_4.set_name('Rx-2');
dev_4.set_coordinate([100,100,0]);
dev_4.set_marker('mo');

% Create network.
net = network_mfm();

% Add devices to network as source-destination pairs.
net.add_source_destination(dev_1,dev_2);
net.add_source_destination(dev_3,dev_4);

% Automatically populate links based on source-destination pairs.
net.populate_links_from_source_destination();

% Set network-wide channel and path loss models.
net.set_path_loss(path_loss_object);
net.set_channel(channel_object);

% Finish network setup.
net.set_symbol_bandwidth(symbol_bandwidth_Hz);
net.set_propagation_velocity(propagation_velocity_meters_per_sec);
net.set_carrier_frequency(carrier_frequency_Hz);
net.set_num_streams(num_streams);
net.set_transmit_power(transmit_power_dBm,'dBm');
net.set_noise_power_per_Hz(noise_power_per_Hz_dBm_Hz,'dBm_Hz');

% View the network.
net.show_2d();

% Invoke a realization of the entire network.
net.realization();

% Compute and supply channel state information to each device.
net.compute_channel_state_information();
net.supply_channel_state_information();

% Configure all transmitters and receivers.
net.configure_transmitter('eigen');
net.configure_receiver('mmse-int');

% Compute received signals based on realization and configuration.
net.compute_received_signals();

% Report mutual information of the two desired links.
mi_12 = net.report_mutual_information(dev_1,dev_2);
mi_34 = net.report_mutual_information(dev_3,dev_4);

disp(['M.I. (1) --> (2): ' num2str(mi_12) ' bps/Hz']);
disp(['M.I. (3) --> (4): ' num2str(mi_34) ' bps/Hz']);

% Report symbol estimation error of the two desired links.
[err_12,nerr_12] = net.report_symbol_estimation_error(dev_1,dev_2);
[err_34,nerr_34] = net.report_symbol_estimation_error(dev_3,dev_4);

disp(['Norm. symb. est. error: (1) --> (2): '...
 num2str(10*log10(nerr_12)) ' dB']);
disp(['Norm. symb. est. error: (3) --> (4): '...
 num2str(10*log10(nerr_34)) ' dB']);
\end{verbatim}

\subsection{Output}
\begin{verbatim}
M.I. (1) --> (2): 9.7535 bps/Hz
M.I. (3) --> (4): 10.7976 bps/Hz
Norm. symb. est. error: (1) --> (2): -5.8628 dB
Norm. symb. est. error: (3) --> (4): -8.5364 dB
\end{verbatim}
